# Supplementary material for: Long-range Rydberg molecule Rb$_2$: Two-electron \textit{R}-matrix calculations at intermediate internuclear distances
Source: arXiv:2003.13495 source file (2020-11-11)
Supplement: Supplementary file 1 [file supplm.pdf]

# Supplemental Online Information

## I. REPRESENTATION OF Rb AND $Rb^+$

In the two-electron $R$-matrix method, the positive atomic core of the neutral perturber $A$ is represented by a potential $V_A(r)$. Its parameters are optimized to reproduce the energies $\varepsilon_{nl}$ of the ground and excited states of the neutral atom, where $n$ and $l$ denote the principal quantum number and angular momentum of the valence electron, respectively.

Following Marinescu *et al.* [1], an $l$-dependent potential $V_A^{(l)}(r)$ was used for $l \leq 3$ to represent the positive core $Rb^+$. Although the $l$-dependence of $V_A^{(l)}(r)$ was not explicitly assumed in TC, it does not represent any practical difficulty.

The model potential utilized in the calculations presented in this work is

$$V_A^{(l)}(r) = -\frac{1 + (Z-1)e^{-\beta_{1l}r} + \beta_{2l}re^{-\beta_{3l}r}}{r} - \frac{\alpha_{dc}}{2r^4}\left[1 - e^{-(r/r_{cl})^6}\right], \qquad (1)$$

where $Z = 37$ is the nuclear charge of Rb, $\alpha_{dc} = 9$ a.u. is the static dipole polarizability of $Rb^+$ [2], $\beta_{1l}$, $\beta_{2l}$, $\beta_{3l}$ and $r_{cl}$ are the fitting parameters. The potential $V_A^{(l)}(r)$ was optimized for several lowest states with $l = 0 \ldots 3$ to match the corresponding experimental energies [3].

The energy splitting of the excited states due to the spin-orbit interaction is larger than the accuracy with which these states can be obtained using $V_A^{(l)}(r)$. Since the spin-orbit coupling is not considered in this study, the pairs of the experimental energies [3] within the $nl$ manifold with $j = l \pm 1/2$ were $j$-averaged (for $l > 0$) and subsequently used to fit $V_A^{(l)}(r)$. The parameters in Eq. (1) were fitted to match lowest 6, 5, 5, 5 $j$-averaged energies of the states with $l = 0, 1, 2, 3$ respectively. The eigenenergies of the states with $l > 3$ are very close to those of the hydrogen atom and the corresponding model potential was set to $V_A^{(l>3)}(r) = -1/r$.

The optimization of $V_A^{(l)}(r)$ was for the rubidium atom performed in the same way as was discussed by Tarana and Čurík [4] for lithium. The obtained values of the parameters are summarized in Table I. The largest difference between the $j$-averaged experimental energy [3] and corresponding value obtained using $V_A^{(l)}(r)$ among the states used for the optimization, was smaller than $0.5\,\text{cm}^{-1}$.

TABLE I. Optimized values of the parameters in Eq. (1).

| $l$ | $\beta_{1l}$ | $\beta_{2l}$ | $\beta_{3l}$ | $r_{cl}$ |
|---|---|---|---|---|
| 0 | 4.58399 | 16.3777 | 1.91381 | 1.23606 |
| 1 | 4.67960 | 17.6441 | 1.94827 | 1.31018 |
| 2 | 4.40538 | 15.5548 | 1.95719 | 1.20402 |
| 3 | 3.93385 | 27.7401 | 2.19395 | 2.58766 |

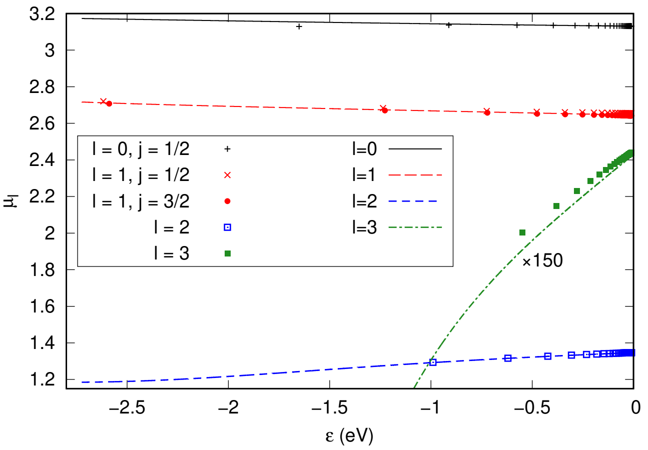


FIG. 1. Quantum defects of Rb as functions of negative energy for $l = 0 \ldots 3$. The lines represent the values calculated using the model potential $V_A^{(l)}(r)$. The experimental data measured by Lorenzen and Niemax [5] are plotted with points. For $l = 1$, the experimental quantum defects are plotted for both $j = 1/2$ and $j = 3/2$.

In addition to the low lying states of Rb, $V_A^{(l)}(r)$ yields accurate energies of the higher excited states that were not involved in the optimization procedure. This was verified by the calculation of the corresponding energy-dependent quantum defects $\mu_l(\varepsilon)$ for the negative energies and by their comparison with the experimental results previously published by Lorenzen and Niemax [5]. Since the positive core $B$ of the Rydberg atom is in the two-electron $R$-matrix method represented by the quantum defects, this agreement shows that both cores $A$ and $B$ are treated consistently with each other.

In addition to the potential $V_A^{(l)}$ and electron-electron repulsion, the dielectronic term [6, 7] was added to the two-electron Hamiltonian in the $R$-matrix calculations of the PECs to treat the interaction between the Rydberg electron and neutral perturber more accurately. This term accounts for the interaction between the valence and Rydberg electrons via the dipole and quadrupole moments induced on the core $A$. The explicit form of this term utilized in this study as well as the optimization of the parameters are identical to those described by Tarana and Čurík [4] for the lithium atom. In addition to the static dipole polarizability of the $Rb^+$ core $\alpha_{dc} = 9$ a.u. [2], the dielectronic correction is parametrized by the quadrupole polarizability of $Rb^+$ $\alpha_{qc} = 35.4$ a.u. [8] and by the cutoff radius $\rho_c = 1$ a.u. optimized to accurately reproduced the electron affinity of Rb.

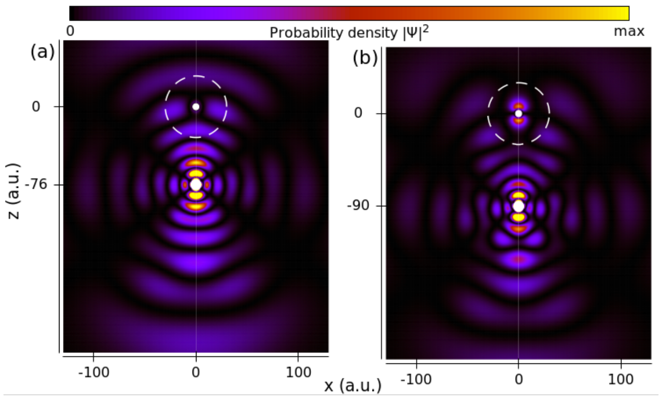


FIG. 2. Two-dimensional maps of the Rydberg electron probability densities in the perturbed state $11d$. The perturber is located in the center of the coordinate system and the white circle denotes the $R$-matrix sphere. The internuclear distances are marked on the vertical axes and corresponding points on the PECs are labeled in Fig. 3 of the article.

## II. DETAILS OF THE $B$-SPLINE BASIS USED INSIDE THE $R$-MATRIX SPHERE

The radial basis set of 86 $B$-splines of the 8th order was defined inside the $R$-matrix sphere on knot sequence spanning the interval $[0, r_0]$. It was divided into three subintervals with equidistant separation of the knot points in each of them: 10 knots were used in the subinterval $[0, 1/37]$ a.u., set of 10 knots was used in the subinterval $[1/37, 2]$ a.u. and 60 points uniformly spanned the remaining interval to the surface of the $R$-matrix sphere.

## III. WAVE FUNCTIONS OF THE RYDBERG ELECTRON

Figure 2 shows the probability densities of the Rydberg electron for the state with the asymptote $5s + 11d$. The maps for other states with the asymptotes $5s + ns$, $5s + nd$ and $5s + nf$ show the same qualitative features. As can be seen in Fig. 2, the perturber affects the probability density of the Rydberg electron most significantly locally inside the $R$-matrix sphere. Outside, the wave functions approximately retain their atomic character. At internuclear distances $R$ corresponding to the local minima of the PECs, the $s$-wave component (with respect to the perturber) predominates the wave function inside the sphere [see Fig. 2 (a)]. Similarly, at internuclear distances $R$ where the PECs attain their local maxima, the wave function of the Rydberg electron inside the sphere shows predominately $p$-wave character [see Fig. 2 (b)]. This fits in the picture provided by the zero-range potential model where the $s$-wave and $p$-wave component (with respect to the center of the perturber) dominate at the values of $R$ corresponding to the local maximum of the value and of the gradient of the atomic Rydberg wave function, respectively.

The Rydberg wave functions obtained from the finite-range one-electron approach used in this work can technically be evaluated everywhere in the space. However, note that the small vicinities of both atomic centers were excluded from all the plots of the probability densities presented in this work. The Coulomb Green's function with the short-range correction involves the irregular Whittaker function. Therefore, when it is used to propagate the solution of the Schrödinger equation, it shows an unphysical increase in the small vicinity of the Rydberg core ($\approx 4$ a.u. for $Rb^+$). The wave function in the close vicinity of the perturber core ($\approx 4$ a.u. for Rb) shows rapid unphysical oscillations with large amplitudes due to very attractive character of the model potentials [9] near the center. Both these regions are in reality occupied by the electrons of the corresponding atomic core. Therefore, the wave functions do not have single-particle character there and they are not presented in this work.


[1] M. Marinescu, H. R. Sadeghpour, and A. Dalgarno, Dispersion coefficients for alkali-metal dimers, Phys. Rev. A **49**, 982 (1994).

[2] S. Chattopadhyay, B. K. Mani, and D. Angom, Electric dipole polarizabilities of alkali-metal ions from perturbed relativistic coupled-cluster theory, Phys. Rev. A **87**, 042520 (2013).

[3] J. E. Sansonetti, Wavelengths, Transition Probabilities, and Energy Levels for the Spectra of Rubidium (Rb I through Rb XXXVII), J. Phys. Chem. Ref. Data **35**, 301 (2006); Erratum: "Wavelengths, Transition Probabilities, and Energy Levels for the Spectra of Rubidium (Rb I through Rb XXXVI)" [J. Phys. Chem. Ref. Data 35, 301–421 (2006)], **37**, 1183 (2008).

[4] M. Tarana and R. Čurík, $R$-matrix calculations of electron collisions with a lithium atom at low energies, Phys. Rev. A **99**, 012708 (2019).

[5] C.-J. Lorenzen and K. Niemax, Quantum Defects of the $n^2P_{1/2,3/2}$ Levels in $^{39}$K I and $^{85}$Rb I, Phys. Scr. **27**, 300 (1983).

[6] C. D. H. Chisholm and U. Öpik, A simplified Hartree-Fock procedure for atoms with two electrons outside closed shells, Proc. Phys. Soc. **83**, 541 (1964).

[7] C. Bahrim and U. Thumm, Low-lying $^3P^o$ and $^3S^e$ states of $Rb^-$, $Cs^-$, and $Fr^-$, Phys. Rev. A **61**, 022722 (2000).

[8] R. M. Sternheimer, Quadrupole polarizabilities of various ions and the alkali atoms, Phys. Rev. A **1**, 321 (1970).

[9] A. A. Khuskivadze, M. I. Chibisov, and I. I. Fabrikant, Adiabatic energy levels and electric dipole moments of Rydberg states of $Rb_2$ and $Cs_2$ dimers, Phys. Rev. A **66**, 042709 (2002).
